# Supplementary material for: Chirotactic response of microswimmers in fluids with odd viscosity
Source: arXiv:2405.01506 ancillary file (2024-08-08)
Supplement: Supplementary file 1 [file SupplementalMaterial.pdf]

# Chirotactic response of microswimmers in fluids with odd viscosity
*Supplemental Material*

Yuto Hosaka,[1,*] Michalis Chatzittofi,[1] Ramin Golestanian,[1,2,†] and Andrej Vilfan[1,3,‡]

[1] *Max Planck Institute for Dynamics and Self-Organization (MPI-DS), Am Fassberg 17, 37077 Göttingen, Germany*
[2] *Rudolf Peierls Centre for Theoretical Physics, University of Oxford, Oxford OX1 3PU, United Kingdom*
[3] *Jožef Stefan Institute, 1000 Ljubljana, Slovenia*

## DEFINITION OF THE EULER ANGLES

To describe the angular dynamics of a chiral microswimmer with an intrinsic angular velocity determined in the body frame, it is convenient to work in the swimmer-fixed frame with the basis $(\mathbf{e}_1, \mathbf{e}_2, \mathbf{e}_3)$ oriented such that $\mathbf{e}_3 \equiv \mathbf{p}$. We describe the rotation of the swimmer relative to the laboratory frame with the basis $(\mathbf{e}_x, \mathbf{e}_y, \mathbf{e}_z)$, where $\mathbf{e}_z \equiv \mathbf{e}$, using the Euler angles $(\phi, \theta, \psi)$ [S1] [see Fig. 3(a) in the main text]. The rotation follows the $zxz$-convention, which is composed of a rotation of angle $\phi$ about $\mathbf{e}_z$, a rotation of $\theta$ about the $x$ axis of the resulting reference frame and, a rotation of $\psi$ about the body fixed axis $\mathbf{e}_3$. Then the rotation matrix $\mathbf{R}$, which transforms the laboratory frame basis vectors to the body-fixed basis vectors (active transformation) via the relation

$$\left(\mathbf{e}_1 \ \mathbf{e}_2 \ \mathbf{e}_3\right) = \mathbf{R} \cdot \left(\mathbf{e}_x \ \mathbf{e}_y \ \mathbf{e}_z\right), \tag{S1}$$

is given by [S1]

$$\mathbf{R} = \begin{pmatrix} \cos\phi\cos\psi - \sin\phi\cos\theta\sin\psi & -\cos\phi\sin\psi - \sin\phi\cos\theta\cos\psi & \sin\phi\sin\theta \\ \sin\phi\cos\psi + \cos\phi\cos\theta\sin\psi & -\sin\phi\sin\psi + \cos\phi\cos\theta\cos\psi & -\cos\phi\sin\theta \\ \sin\theta\sin\psi & \sin\theta\cos\psi & \cos\theta \end{pmatrix}. \tag{S2}$$

The inverse transformation is given by

$$\left(\mathbf{e}_x \ \mathbf{e}_y \ \mathbf{e}_z\right) = \mathbf{R}^T \cdot \left(\mathbf{e}_1 \ \mathbf{e}_2 \ \mathbf{e}_3\right). \tag{S3}$$

In particular, $\mathbf{e}_z$ can be expressed in the swimmer frame as $\mathbf{e}_z = \sin\theta\sin\psi\mathbf{e}_1 + \sin\theta\cos\psi\mathbf{e}_2 + \cos\theta\mathbf{e}_3$.

The angular velocity of the swimmer can be expressed with the derivatives of the Euler angles as [S1]

$$\mathbf{\Omega} = (\dot\phi\sin\theta\sin\psi + \dot\theta\cos\psi)\mathbf{e}_1 + (\dot\phi\sin\theta\cos\psi - \dot\theta\sin\psi)\mathbf{e}_2 + (\dot\phi\cos\theta + \dot\psi)\mathbf{e}_3. \tag{S4}$$

## APPROXIMATE EXPRESSION FOR THE CRITICAL ANGULAR VELOCITY $\Omega^{\mathrm{e}}_{\mathrm{c}}$

The critical angular velocity, at which the saddle-node bifurcation takes place in the dynamical system determined by Eq. (12) from the main text can be derived analytically in the limit $|\lambda| \ll 1$. The fixed points $(\bar\theta, \bar\psi)$ correspond to the solutions of equations $\dot\theta = 0$ and $\dot\psi = 0$, leading to the conditions

$$0 = \frac{3g_2(\lambda)B_2}{10a}\sin(2\bar\theta) + \Omega^{\mathrm{e}}\sin\gamma\cos\bar\psi, \tag{S5}$$

$$0 = \frac{3g_1(\lambda)B_2}{5a}\cos\bar\theta + \Omega^{\mathrm{e}}\left(\cos\gamma - \frac{\sin\gamma\sin\bar\psi}{\tan\bar\theta}\right). \tag{S6}$$

Because $g_2(\lambda) \ll g_1(\lambda)$, Eqs. (S5) and (S6) can only be solved simultaneously if $\cos\bar\psi \approx 0$. With $B_2 < 0$ and $\gamma < \pi/2$ (the situation shown in Fig. 3 in the main text), the saddle-node bifurcation takes place between two fixed points at $\bar\psi \approx 3\pi/2$, whereas the solution $\bar\psi \approx \pi/2$ gives a single spiral source. We therefore choose $\bar\psi = 3\pi/2$ to analyze the bifurcation. Equation (S6) then simplifies to

$$\Omega^{\mathrm{e}}(\bar\theta) = -\frac{3\lambda B_2}{40a}\frac{\sin(2\bar\theta)}{\sin(\gamma + \bar\theta)}. \tag{S7}$$

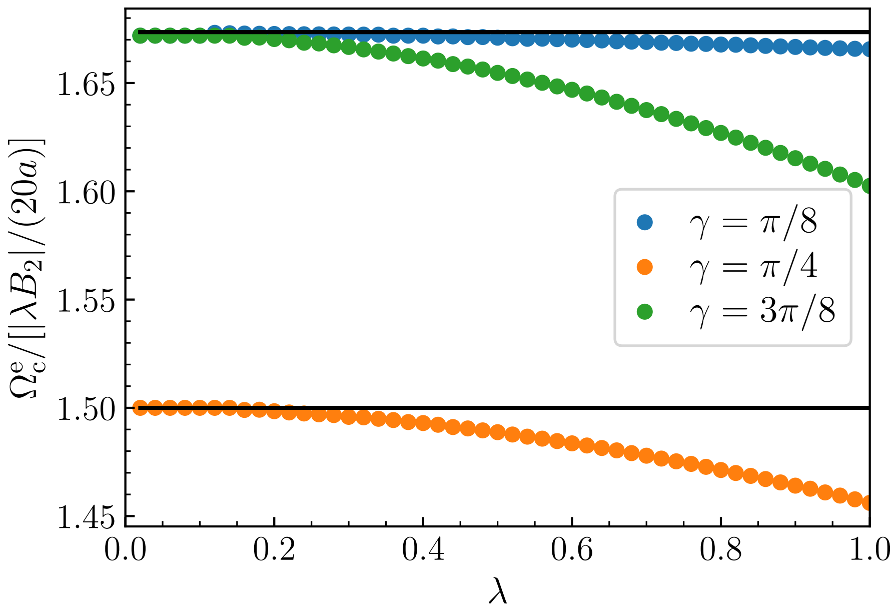


FIG. S1. Numerical solution for the critical angular velocity. The rescaled critical angular velocity $\Omega_c^e$ is calculated as a function of the odd viscosity ratio $\lambda$ for three values of the angle $\gamma$. The solid lines represent the analytical approximation (S9).

For a fixed $\Omega^e$, Eq. (S7) is solved by either 1 or 3 values of $\bar{\theta}$. The saddle-node bifurcation, at which 2 solutions vanish, corresponds to a local maximum of $\Omega^e(\bar{\theta})$. From the condition $\partial\Omega^e(\bar{\theta})/\partial\bar{\theta} = 0$, we obtain the position in phase space at which the bifurcation takes place

$$(\bar{\theta}, \bar{\psi}) = \left(\arctan\left(\tan^{1/3}\gamma\right), \frac{3}{2}\pi\right), \tag{S8}$$

which gives the critical value

$$\Omega_c^e = -\frac{3\lambda B_2}{20a}(\sin^{2/3}\gamma + \cos^{2/3}\gamma)^{-3/2}, \tag{S9}$$

for $0 < \gamma < \pi/2$. Expression (S9) has a minimum at $\gamma = \pi/4$. The lowest possible critical angular frequency is $\Omega_c^e = (3/2)|\lambda B_2|/(20a)$.

For larger $\lambda$, the critical angular velocity can be determined numerically by analyzing the number of fixed points in the dynamical system. Figure S1 shows $\Omega_c^e$ as a function of $\lambda$ for three values of $\gamma$. The analytical expression is exact in the limit $\lambda \ll 1$ and the deviation stays within a few percent up to $\lambda = 1$.

* yuto.hosaka@ds.mpg.de
† ramin.golestanian@ds.mpg.de
‡ andrej.vilfan@ds.mpg.de

[S1] H. Goldstein, C. Poole, and J. Safko, *Classical Mechanics*, 3rd ed. (Pearson, Boston MA, 2001).
